# Supplementary material for: Monocular Depth Estimators: Vulnerabilities and Attacks
Source: arXiv:2005.14302 source file (2020-05-28)
Supplement: Supplementary file 1 [file blackbox_patch_relabs.tex]

%\begin{table*}
	\begin{tabular}{l|c|c|c}
		\hline
		Methods & Clean & \multicolumn{2}{c}{Attacked} \\
		\cline{2-4}
		& Absrel         & Absrel   & Rel (\%)   \\
		\hline
		SFM      & 0.1755       & 0.1962   & 12    \\
		B2F      & 0.1358       & 0.1477   & 5    \\
		SCSFM    & 0.1283       & 0.1477   & 16    \\
		Mono1    & 0.1095       & 0.12     & 10     \\
		Mono2    & 0.1123       & 0.116    & 4    \\
		\hline
	\end{tabular}
%	\caption{Black-box Patch Attack $72 \times 72$. Absolute relative error.}
%	\label{blackbox_patch_relabs}
%\end{table*}
