# Supplementary material for: Monocular Depth Estimators: Vulnerabilities and Attacks
Source: arXiv:2005.14302 source file (2020-05-28)
Supplement: Supplementary file 2 [file blackbox_pert_relabs.tex]

%\begin{table*}
	\begin{tabular}{l|c|c|c}
		\hline
		Methods & Clean & \multicolumn{2}{c}{Attacked} \\
		\cline{2-4}
		& Absrel         & Absrel   & Rel (\%)   \\
		\hline
		SFM      & 0.1755       & 0.1842    & 5    \\
		B2F      & 0.1358       & 0.1688    & 25    \\
		SCSFM    & 0.1283       & 0.161     & 26    \\
		Mono1    & 0.1095       & 0.124     & 14     \\
		Mono2    & 0.1123       & 0.1452    & 30    \\
		\hline
	\end{tabular}
%	\caption{Black-box Perturbation Attack $\eta=0.05$. Absolute relative error.}
%	\label{blackbox_pert_relabs}
%\end{table*}
